# Supplementary material for: Merging of Soap Bubbles and Why Surfactant Matters
Source: arXiv:1911.03175 ancillary file (2020-01-22)
Supplement: Supplementary file 1 [file SM.pdf]

# Supplementary Material for Merging of Soap Bubbles and Why Surfactant Matters

Patricia Pfeiffer and Claus-Dieter Ohl
*Institute for Physics, Otto von Guericke University Magdeburg, Magdeburg 39106, Germany**

Qingyun Zeng
*Division of Physics and Applied Physics, School of Physical and Mathematical Sciences, Nanyang Technological University, 637371 Singapore, Singapore*

Beng Hau Tan
*Low Energy Electronic Systems, Singapore-MIT Alliance for Research and Technology, Singapore 138602, Singapore*

## I. EXPERIMENTAL SETUP

Figure S1 shows the experimental setup.

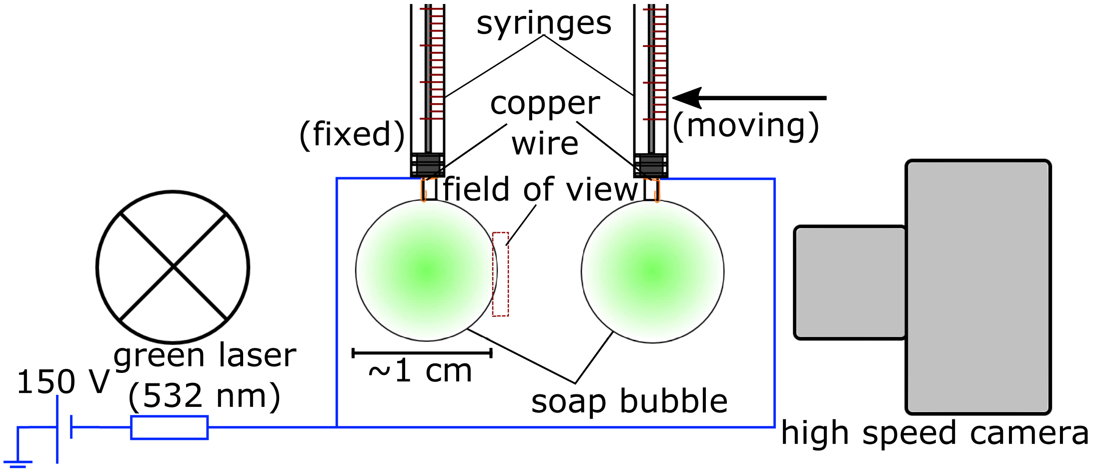


Figure S 1. Experimental setup for studying the merging of two soap bubbles. The soap bubbles are inflated with a syringe each. One is fixed and the other syringe is moved slowly towards the second until the bubbles touch each other. The merging is monitored by imaging head-on through the bubbles with a high speed camera.

## II. DETAILS OF SIMULATION

In the simulation we do not compute the dynamics of the merged film point directly, instead we conduct a simulation to solve the dynamics of a merged film ring, which is considered to have a similar initial acceleration with the merged point. Therefore we simplify the simulation domain to be axisymmetric, see figure S2. The computed mesh is refined to a spacing $\Delta x \approx 30\,\mathrm{nm}$ in the area where the soap film is located. The air-liquid interface is captured using the compressible volume of fluid (VoF) method in OpenFOAM [1]. The numerical model also takes into account surface tension, viscosity and compressibility. Details of the governing equation and numerical algorithm can be found in Zeng et al. [2].

---

* patricia.pfeiffer@ovgu.de

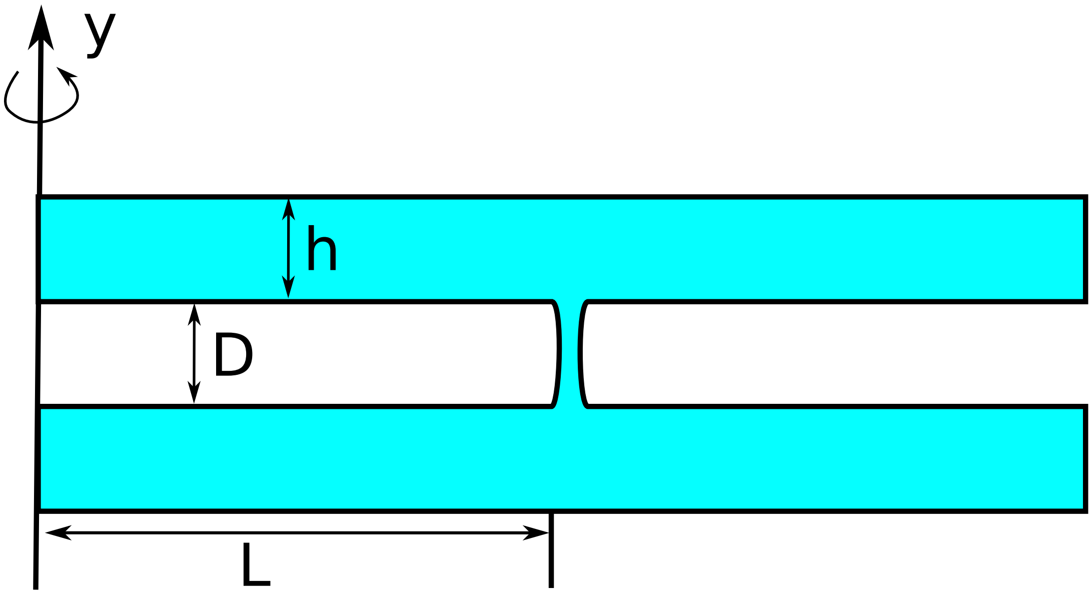


Figure S 2. Sketch of the simulation domain. The soap film is coded in cyan with a thickness of h=5.5 µm and a radius of L=100 µm. The height of the air dimple is D=1.6 µm. Note that the vertical scale is strongly stretched. Surface tension $\sigma$ =0.025 N/m.

Figure S3 shows snapshots of the simulations. The dimple is located on the right side of the liquid bridge. The merged film expands in both directions.

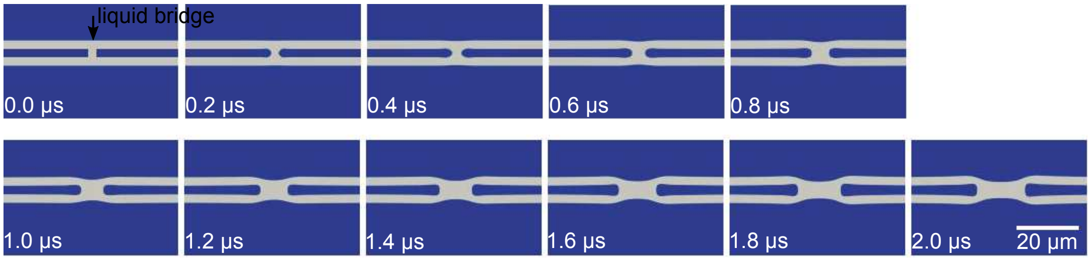


Figure S 3. Snapshots of the simulations of the growth of the rim. The dimple is located on the right side of the liquid bridge.

[1] H. G. Weller, G. Tabor, H. Jasak, and C. Fureby, Comput. Phys. **12**, 620 (1998).
[2] Q. Zeng, S. R. Gonzalez-Avila, S. Ten Voorde, and C.-D. Ohl, J. Fluid Mech. **846**, 916 (2018).
